# Supplementary material for: Laboratory-scale Perpendicular Collisionless Shock Generation and Ion Acceleration in Magnetized Head-on Colliding Plasmas
Source: arXiv:2405.14081 source file (2024-05-23)
Supplement: Supplementary file 1 [file supplement0505.pdf]

# Supplemental Material: Magnetized Scenario with a Magnetized Ambient Plasma


P. Liu,[1] D. Wu,[2,*] D. W. Yuan,[3] Z. M. Sheng,[1] X. T. He,[1] and J. Zhang[2,†]

[1]*Institute for Fusion Theory and Simulation, School of Physics, Zhejiang University, Hangzhou 310058, China*
[2]*Key Laboratory for Laser Plasmas and School of Physics and Astronomy, Collaborative Innovation Center of IFSA (CICIFSA), Shanghai Jiao Tong University, Shanghai 200240, China*
[3]*Key Laboratory of Optical Astronomy, National Astronomical Observatories, Chinese Academy of Sciences, Beijing 100012, China*



(Dated: May 7, 2024)


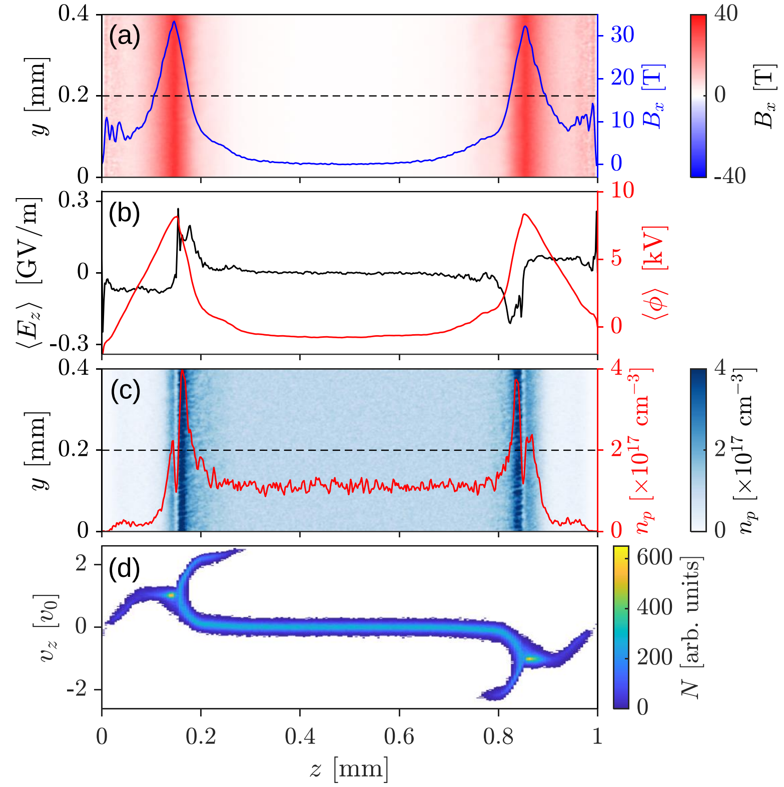


Figure S1. (a) Self-generated magnetic field distribution, where the blue line represents the profile of $B_x$ along the black line. (b) Longitudinal electric field $\langle E_z \rangle$ and electric potential $\langle \phi \rangle$ profiles, where $\langle \cdot \rangle$ represents averaging over the $y$ direction. (c) Spatial density distribution of the ambient protons, where the red line represents the profile of $n_p$ along the black line. (d) Phase space $(z - v_z)$ distributions of the ambient protons. All above results are at simulation time $t = 120$ ps.

It is noteworthy that the magnetized shock driven by counter-streaming plasma flows is distinct from that created through the interaction of injected flow with a magnetized ambient plasma, and the latter configurations are more common in previous astrophysical experiments [1–6]. Inspired by this experimental setup, in this work, we also perform a simulation including a ambient plasma, which is created by laser pre-ablating polyethylene ($CH_2$) target [2, 3]. The density of ambient plasma is $n_e = 4 \times 10^{17}$ cm$^{-3}$, and other parameters are the same as that of Fig. 3 in the main text.

When a injected flow interacts with the magnetized low-density ambient plasma, We demonstrate that a magnetized shock is formed in Figs. S1(a)-S1(c), exhibiting a distinct boundary between the downstream and upstream regions in terms of the self-generated magnetic field $B_x$, the longitudinal electric field $E_z$, and the proton density $n_p$. The maximum amplitude of magnetic field $B_m = B_x + B_0$ grows from $\sim 1.5B_0$ to $\sim 2.7B_0$, which is much smaller than


* dwu.phys@sjtu.edu.cn
† jzhang@iphy.ac.cn

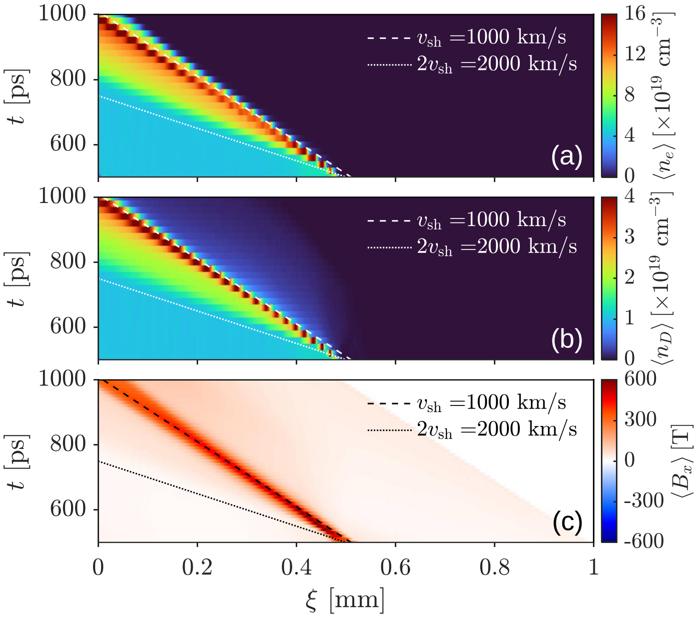


Figure S2. Spatiotemporal structures of electron density (a), deuteron density (b), and self-generated magnetic field (c). The dashed lines depicts the trajectory of the shock front with the velocity of $v_{\rm sh}$, and the dotted lines represents the trajectory of reflected particles with the velocity of $2v_{\rm sh}$; $\langle\cdot\rangle$ represents averaging over the $y$ direction. Here, $\xi = z - v_0(t - t')$ when $t \geq t'$ with $t' = 500$ ps being the moment of colliding between two flows.

that produced by the head-on colliding plasmas. The density jump, $\delta = n_{\rm ds}/n_{\rm us} \sim 4.0$, is close to the upper limit of the prediction of the Rankine-Hugoniot equations, where $n_{\rm us}$ and $n_{\rm ds}$ are the upstream and downstream densities of the shock. Additionally, a ion reflection is clearly seen in the $z - v_z$ phase space [see Fig. S1(d)], which is due the electrostatic cross-shock potential produced by longitudinal peaked electric field.

After the colliding of two pre-magnetized plasma flows, it is found that the low-density background plasma has a negligible impact on the shock formation and associated the ion acceleration, with the underlying physical processes closely resembling those depicted in Fig. 3 of the main text, as shown in Fig. S2.


[1] D. B. Schaeffer, E. T. Everson, D. Winske, C. G. Constantin, A. S. Bondarenko, L. A. Morton, K. A. Flippo, D. S. Montgomery, S. A. Gaillard, and C. Niemann, Generation of magnetized collisionless shocks by a novel, laser-driven magnetic piston, Phys. Plasmas **19**, 070702 (2012).

[2] D. B. Schaeffer, W. Fox, D. Haberberger, G. Fiksel, A. Bhattacharjee, D. H. Barnak, S. X. Hu, and K. Germaschewski, Generation and evolution of high-mach-number laser-driven magnetized collisionless shocks in the laboratory, Phys. Rev. Lett. **119**, 025001 (2017).

[3] D. B. Schaeffer, W. Fox, R. K. Follett, G. Fiksel, C. K. Li, J. Matteucci, A. Bhattacharjee, and K. Germaschewski, Direct observations of particle dynamics in magnetized collisionless shock precursors in laser-produced plasmas, Phys. Rev. Lett. **122**, 245001 (2019).

[4] D. B. Schaeffer, W. Fox, J. Matteucci, K. V. Lezhnin, A. Bhattacharjee, and K. Germaschewski, Kinetic simulations of piston-driven collisionless shock formation in magnetized laboratory plasmas, Phys. Plasmas **27**, 042901 (2020).

[5] W. Yao, A. Fazzini, S. N. Chen, K. Burdonov, P. Antici, J. Béard, S. Bolaños, A. Ciardi, R. Diab, E. D. Filippov, *et al.*, Laboratory evidence for proton energization by collisionless shock surfing, Nat. Phys. **17**, 1177 (2021).

[6] W. Yao, A. Fazzini, S. N. Chen, K. Burdonov, P. Antici, J. Béard, S. Bolaños, A. Ciardi, R. Diab, E. D. Filippov, *et al.*, Detailed characterization of a laboratory magnetized supercritical collisionless shock and of the associated proton energization, Matter Radiat. Extremes **7**, 014402 (2021).
